# Supplementary material for: MCDAL: Maximum Classifier Discrepancy for Active Learning
Source: arXiv:2107.11049 source file (2022-02-14)
Supplement: Supplementary file 1 [file 5.supplementary.tex]

% The contents of this supplementary material include additional experimental results, 
% % implementation 
% % details of our model, more qualitative results and
% analysis, and detailed explanations which has been omitted from the main paper due to the space limitation.

% \begin{figure*}[t]
% \centering
%   %\includegraphics[width=1\linewidth]{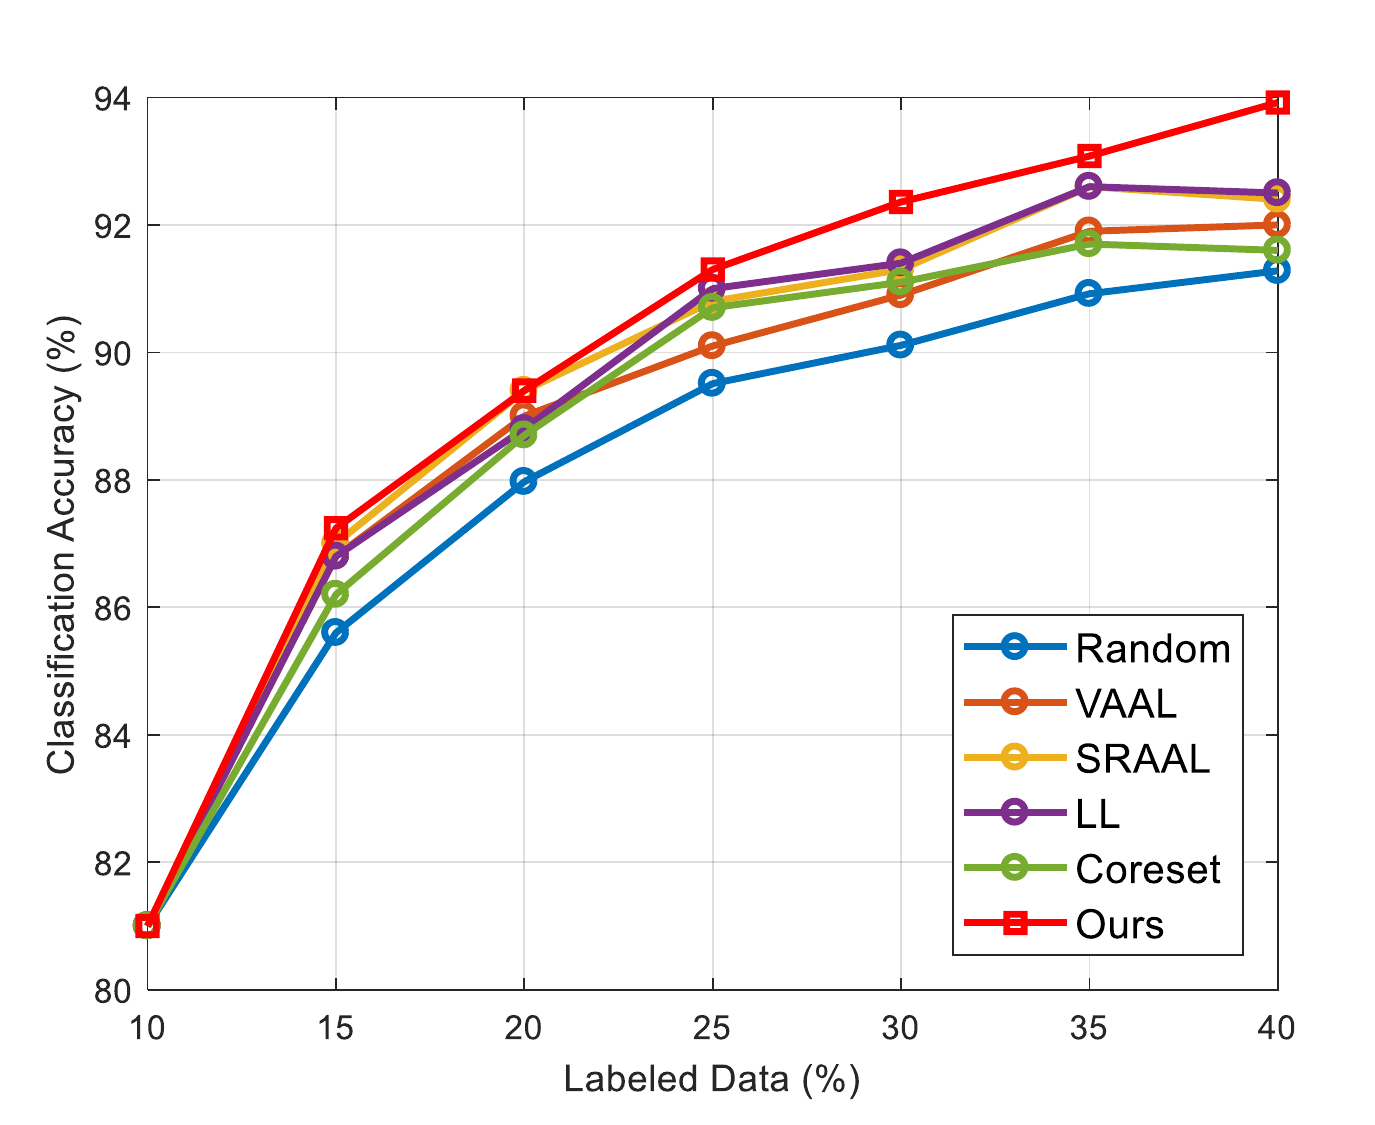}
%   \fbox{\rule{0pt}{2in} \rule{0.9\linewidth}{0pt}}
%   \caption{Comparison in training loss curve between different frameworks (GAN based~\cite{sinha2019variational}, learning loss~\cite{yoo2019learning}, core-set~\cite{sener2017active}, and our framework).\djkim{(to supplementary)}}
% \label{fig:convergence}
% \end{figure*}

\noindent\textbf{Class-aware interpretation.}
The acquisition function in
% ~\Eref{eqn:final} 
Eq. (10)
can be re-written as:
\begin{equation}
%\scriptsize
\begin{split}
    S(x_u) =\Bigg|& \frac{1}{C}\sum_{c=1}^C{|p^c_1(y|x_u) - p^c_2(y|x_u)|} -\\ &\frac{1}{|\mathcal{D}_L|}\sum_{x_l\in\mathcal{D}_L}{\frac{1}{C}\sum_{c=1}^C{|p^c_1(y|x_l) - p^c_2(y|x_l)|}} \Bigg|\\
    =\Bigg| \frac{1}{C}\sum_{c=1}^C \Bigg(&{|p^c_1(y|x_u) - p^c_2(y|x_u)|} -\\ &\frac{1}{|\mathcal{D}_L|}\sum_{x_l\in\mathcal{D}_L}{{|p^c_1(y|x_l) - p^c_2(y|x_l)|}}  \Bigg) \Bigg|.\\
    \end{split}
    %\normalsize
\end{equation}
Here, if we change the absolute value ($|\cdot|$) and by averaging ($\frac{1}{C}\sum_{c=1}^C$), we obtain a variant of our acquisition function as shown:
\begin{equation}
%\scriptsize
\begin{split}
    S(x_u)=\frac{1}{C}\sum_{c=1}^C \Bigg|& {|p^c_1(y|x_u) - p^c_2(y|x_u)|} - \\ &\frac{1}{|\mathcal{D}_L|}\sum_{x_l\in\mathcal{D}_L}{{|p^c_1(y|x_l) - p^c_2(y|x_l)|}} \Bigg|,
    \label{eqn:classwise}
\end{split}
%\normalsize
\end{equation}
which compares the \emph{class-wise} discrepancy difference between labeled sample and the unlabeled dataset.
%The inequality is from Jesnsen's inequality.
This equation can be interpreted that the proposed acquisition function not only measures classifier discrepancy of an unlabeled sample itself, but also measures how the unlabeled sample is far from the distribution in the \emph{class-wise} behavior (probability difference) of the labeled samples which matches with the motivation of GAN based active learning works. 

To test our theory, we perform another ablation study to verify the performance of this method. We run the experiments again on CIFAR-10 to show to verify the performance of this method. 

The comparison is illustrated in \Fref{fig:comparisons}. ``MeanVal'' denotes our final model proposed in Fig.~5. ``MeanVec'' denotes an alternative approach where we compute the class-wise difference between the labeled sample and the unlabeled dataset in \Eref{eqn:classwise}. Finally, ``NoComp'' denotes the baseline where we do not compare the difference between the labeled and the unlabeled dataset and simply using the discrepancy value as the acquisition function (\ie,~$S(x_u)=D(x_l)$).

\begin{figure}[ht]
\centering
  \includegraphics[width=0.95\linewidth]{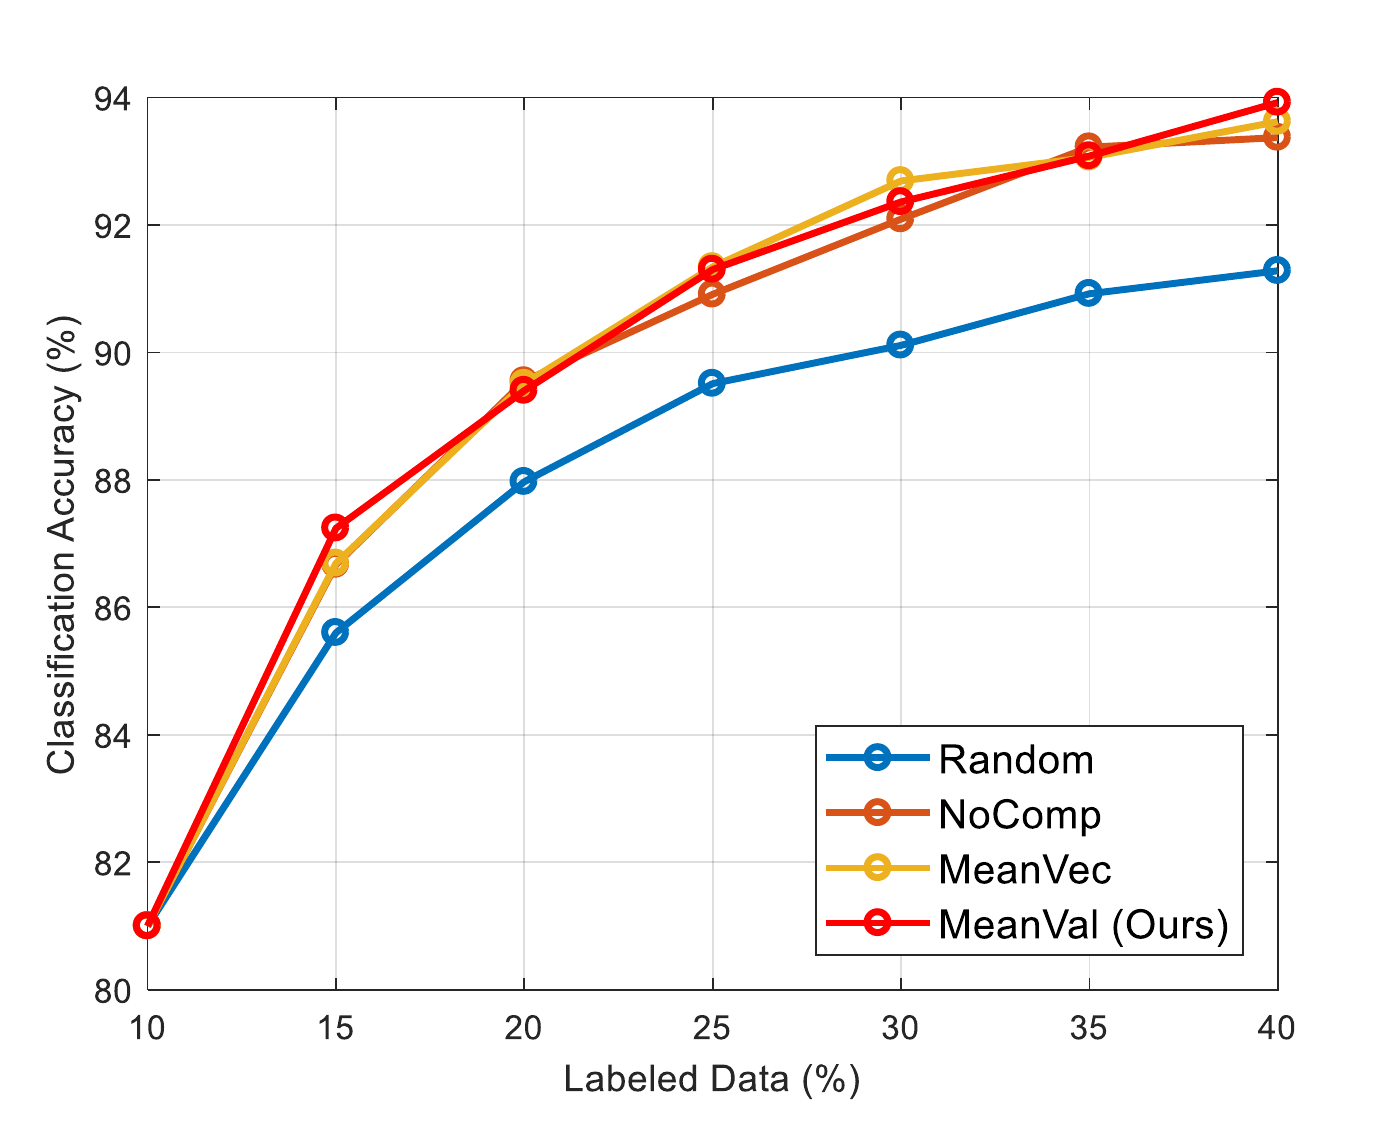}
%   \fbox{\rule{0pt}{2in} \rule{0.9\linewidth}{0pt}}
  \caption{Results from the comparisons of the different class-wise discrepancy measures. The results show minimal differences among all 3 methods, but ``MeanVal'' performs best in most stages, so we decide to use ``MeanVal'' as our baseline method.}
\label{fig:comparisons}
\end{figure}

From \Fref{fig:comparisons}, we can see that although the results seem similar across the board, the general trend is that our method that we decide, ``MeanVal'', performs the best in most stages. For this reason, for the rest of our experiments, we choose this as our baseline and continue through all experiments here.
